# Supplementary material for: Density Decomposition in Dual-Modular Optimization: Markets, Fairness, and Contracts
Source: arXiv:2505.19499 source file (2025-05-26)
Supplement: Supplementary file 1 [file appendix.tex]

\newpage

\section{Appendix}

\subsection{Proof of Fact \ref{fact1}}\label{unimax}

\begin{proof}
Let $S$ be the maximal densest subset with density $\rho=\frac{f(S)}{g(S)}$. Suppose there exists a subset $B$ s.t. $\frac{f(B)}{g(B)}=\rho$.
\begin{align*}
\frac{f(S\cup B)}{g(S\cup B)}&\geq \frac{f(S)+f(B)-f(S\cap B)}{g(S)+g(B)-g(S\cap B)}\\
&=\frac{\rho(g(S)+g(B))-f(S\cap B)}{g(S)+g(B)-g(S\cap B)}\\
&\geq\frac{\rho(g(S)+g(B)-g(S\cap B))}{g(S)+g(B)-g(S\cap B)}\\
&=\rho
\end{align*}
If the equality holds, then the maximality condition will be violated. Otherwise it will contrdict with the densest condition.
\end{proof}

\subsection{Proof of Lemma \ref{lemma1}}\label{decresort}

\begin{proof}
%Special case: $\rho_1>\rho_2$.
%\begin{align*}
%\rho_{2}&=\frac{f(S_{2}\cup U_1)-f(U_1)}{g(S_{2}\cup U_1)-g(U_{1})}\\
%&=\frac{f(S_{2}\cup U_1)-\rho_1g(U_1)}{g(S_{2}\cup U_1)-g(U_{1})}\\
%(\rho_2-\rho_1)g(S_1)&=\rho_2g(S_2\cup S_1)-f(S_2\cup S_1)\\
%&\text{since $S_1$ is the unique maximal densest one.}\\
%&>\rho_2g(S_2\cup S_1)-\rho_1g(S_2\cup S_1)\\
%(\rho_2-\rho_1)g(S_1)&>(\rho_2-\rho_1)g(S_1\cup S_2)
%\end{align*}
%Since $g$ is increasing and positive, then we have $\rho_1>\rho_2$.\\
We show $\rho_{i}>\rho_{i+1}$ for $i=1,\dots,k-1$ as follows.
Define $U_{i}=\cup_{j=0}^{i}S_j$.
\begin{align*}
\rho_{i+1}&=\frac{f(S_{i+1}\cup U_i)-f(U_i)}{g(S_{i+1}\cup U_i)-g(U_{i})}\\
\rho_{i+1}(g(U_{i+1}-g(U_i)))&=f(U_{i+1})-f(U_i)
\end{align*}
Consider $S_{i+1}\cup S_i$ in $V-U_{i-1}$, then we have $\rho_{i}>\frac{f(S_{i+1}\cup S_i\cup U_{i-1})-f(U_{i-1})}{g(S_{i+1}\cup S_i\cup U_{i-1})-g(U_{i-1})}$, which means that $f(U_{i+1})<\rho_{i}(g(U_{i+1})-g(U_{i-1}))+f(U_{i-1})$.
\begin{align*}
\rho_{i+1}(g(U_{i+1})-g(U_i))&=f(U_{i+1})-f(U_i)\\
&<\rho_{i}(g(U_{i+1})-g(U_{i-1}))+f(U_{i-1})-f(U_i)\\
&=\rho_{i}(g(U_{i+1})-g(U_{i-1}))-\rho_i (g(U_{i})-g(U_{i-1}))\\
(\rho_{i+1}-\rho_{i})g(U_{i+1})&<(\rho_{i+1}-\rho_{i})g(U_i)
\end{align*}
Since $g$ is monotone, then we have $\rho_i>\rho_{i+1}$.
\end{proof}
